# Supplementary material for: High-fidelity, high-scalability two-qubit gate scheme for superconducting qubits
Source: arXiv:2006.11860 source file (2020-12-22)
Supplement: Supplementary file 1 [file Supplement.pdf]

# Supplementary Material for
# "High-fidelity, high-scalability two-qubit gate scheme for superconducting qubits"

Yuan Xu,[1,2,3,*] Ji Chu,[4] Jiahao Yuan,[5] Jiawei Qiu,[5] Yuxuan Zhou,[5] Libo Zhang,[1,2,3]
Xinsheng Tan,[4,†] Yang Yu,[4] Song Liu,[1,2,3] Jian Li,[1,2,3,‡] Fei Yan,[1,2,3,§] and Dapeng Yu[1,2,3]

[1]*Shenzhen Institute for Quantum Science and Engineering, Southern University of Science and Technology, Shenzhen, Guangdong, China*
[2]*Guangdong Provincial Key Laboratory of Quantum Science and Engineering, Southern University of Science and Technology, Shenzhen, Guangdong, China*
[3]*Shenzhen Key Laboratory of Quantum Science and Engineering, Southern University of Science and Technology, Shenzhen, Guangdong, China*
[4]*National Laboratory of Solid State Microstructures, Department of Physics, Nanjing University, Nanjing, Jiangsu, China*
[5]*Institute for Quantum Science and Engineering and Department of Physics, Southern University of Science and Technology, Shenzhen, Guangdong, China*

[*]Electronic address: xuy5@sustech.edu.cn
[†]Electronic address: tanxs@nju.edu.cn
[‡]Electronic address: lij33@sustech.edu.cn
[§]Electronic address: yanf2020@mail.sustech.edu.cn;
Y. X. and J. C. contributed equally to this work.

# I. THE DEVICE

## A. Device parameters and experimental setup

The device is fabricated with aluminum on sapphire substrate. Relevant device parameters are summarized in Table S1. The device is mounted inside a dilution refrigerator at a base temperature of about 10 mK. Fridge wiring and measurement circuitry are shown in Fig. S1. We perform the standard circuit-QED measurements.

TABLE S1: Device parameters.

| Parameters (MHz) | $Q_1$ | $Q_2$ |
|---|---|---|
| Resonator frequency ($\omega_{R1}/2\pi$, $\omega_{R2}/2\pi$) | 6955 | 7002 |
| Qubit frequency ($\omega_1/2\pi$, $\omega_2/2\pi$) | 5271 | 4615 |
| Qubit anharmonicity ($\alpha_1/2\pi$, $\alpha_2/2\pi$) | -210 | -240 |
| Coupler frequency (idling) | 6704 | |
| Coupler anharmonicity ($\alpha_c/2\pi$) | $-370$ | |
| Qubit-coupler coupling ($g_{1c}/2\pi$, $g_{2c}/2\pi$) | 122 | 105 |
| Qubit-qubit direct coupling ($g_{12}/2\pi$) | 12 | |
| Single-qubit gate fidelity | 99.84% | 99.90% |
| Readout fidelity | 86% | 85% |

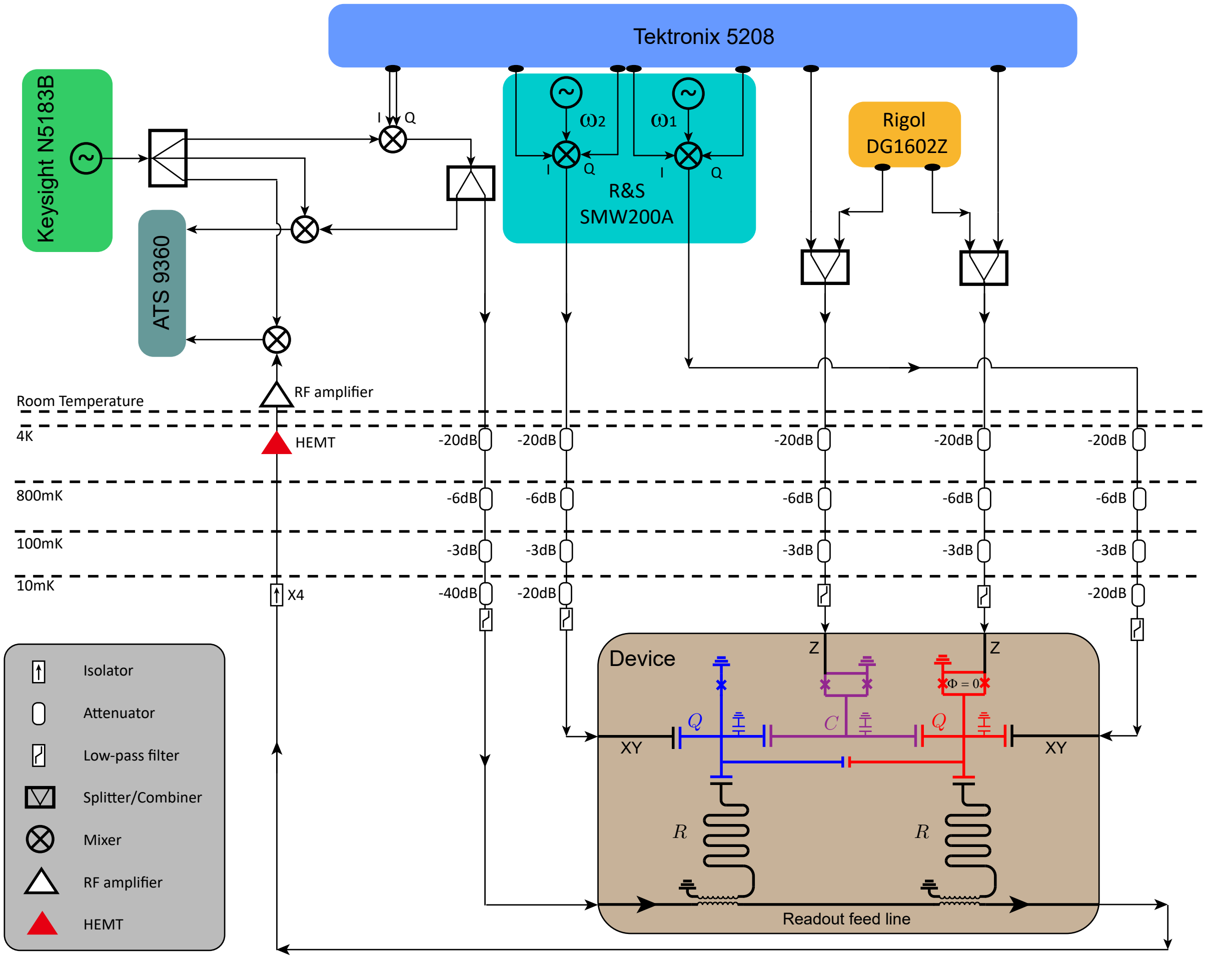


FIG. S1: Wiring diagram and circuit components.

### B. Z crosstalk

In order to use the first qubit $Q_1$ (tunable) as a fixed-frequency qubit, its flux bias has to be set to zero throughout the experiment. Therefore, we characterize and compensate crosstalk of Z control lines between $Q_1$ and the coupler. The crosstalk coefficients (about 8%) are derived from measuring the frequency response to the control lines. However, when $Q_1$ is biased at its maximum frequency as in all subsequent experiments, its frequency becomes insensitive to flux variation, adding extra robustness against crosstalk. Therefore, it is valid to treat $Q_1$ as a fixed-frequency qubit in our experiment.

### C. Coupler spectrum

Due to strong coupling between $Q_2$ and the coupler, there is a frequency shift of $Q_2$ depending on the coupler state. We take advantage of this effect to measure the spectrum of the coupler [1]. The pulse sequence and the measured results are shown in Fig. S2. The two visible avoided crossings correspond to the couplings between the coupler and the two qubits, from which the coupling strengths $g_{1c}$ and $g_{2c}$ can be extracted.

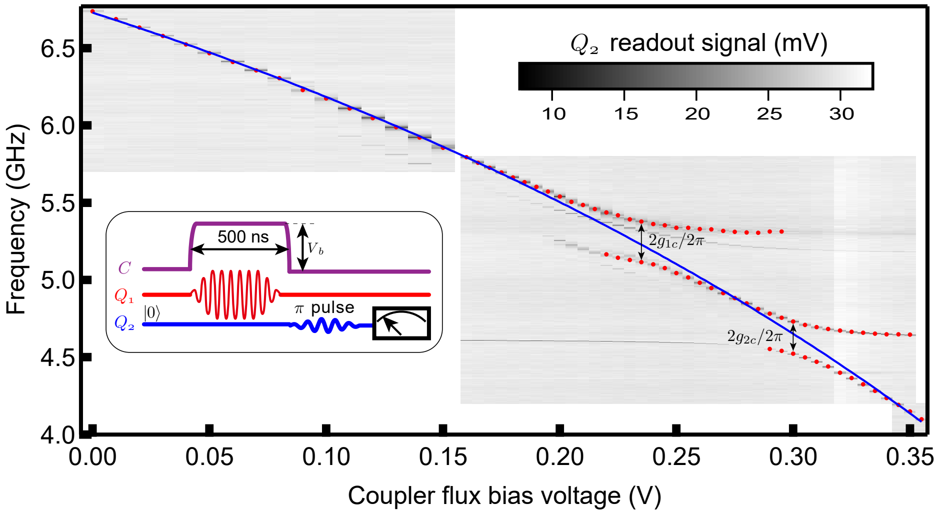


FIG. S2: Measured coupler spectrum with corresponding pulse sequence (inset). The coupler is pulse-biased away from the idling point to a varying amplitude $V_b$ while driven by a microwave pulse applied to the XY control line of $Q_1$. Transitions occur when the drive frequency is on resonance with the pulse-biased coupler frequency. Due to strong coupling between the coupler and $Q_2$, a coupler-state-dependent frequency shift of $Q_2$ can be used to distinguish the coupler state by probing $R_2$ after a selective $\pi$-pulse on $Q_2$. On the greyed color plot, red dashed lines are the measured transitions and the blue solid line is the bare coupler spectrum from fit. The smallest gaps of the two avoided crossings indicate twice the coupling strength.

The coherence of the coupler may be inferred from the its spectral width which is about 10 MHz, equivalent to a $T_2$ time of a few tens of nanoseconds. However, this is very rough estimate, because the spectral width is broadened by the drive. Also, it is important to distinguish the device's local noise from instability of control instrumentation. In general, the AWG used for pulsing the coupler adds extra low-frequency noise. In separate tests, we find that this could limit qubit coherence to only a few hundred nanoseconds.

## II. ENHANCED ADIABATICITY

In general, the adiabatic condition in an adiabatic process between any two states, $|m\rangle$ and $|n\rangle$, is defined by the relation:

$$\beta_{nm} = \left| \frac{\hbar \langle n| \partial H/\partial t |m\rangle}{(E_n - E_m)^2} \right| = \left| \frac{\hbar \langle n|\dot{m}\rangle}{E_m - E_n} \right| \ll 1, n \neq m. \tag{S1}$$

$\beta_{nm}$ quantifies the unwanted transitions. Here, we compare two protocols of adiabatic CZ gate, modulating the frequency of tunable qubits in the conventional fixed-coupling architecture [2, 3] and modulating the frequency of the tunable coupler as done in our work. Summing over all the possible states to which the population transfer, we can rewrite Eq. S1 as

$$\beta_m = \sum_{n \neq m} \left| \frac{\hbar\langle n|\partial H/\partial t|m\rangle}{(E_n - E_m)^2} \right| = \left( \sum_{n \neq m} \left| \frac{\hbar\langle n|\partial H/\partial f|m\rangle}{(E_n - E_m)^2} \right| \right) \left| \frac{\partial f}{\partial t} \right|, \tag{S2}$$

where $f$ denotes the frequency of the tunable coupler. Note that the ramping speed of frequency $|df/dt|$ can be modulated with different pulse waveforms. Normally, $|df/dt| \sim$100 MHz/1 ns in a rapid gate. The energy structure and the corresponding non-adiabaticity factor,

$$\beta = \sum_{n \neq m} \left| \frac{\hbar\langle n|\partial H/\partial f|m\rangle}{(E_n - E_m)^2} \right|, \tag{S3}$$

are then crucial quantities in our discussion.

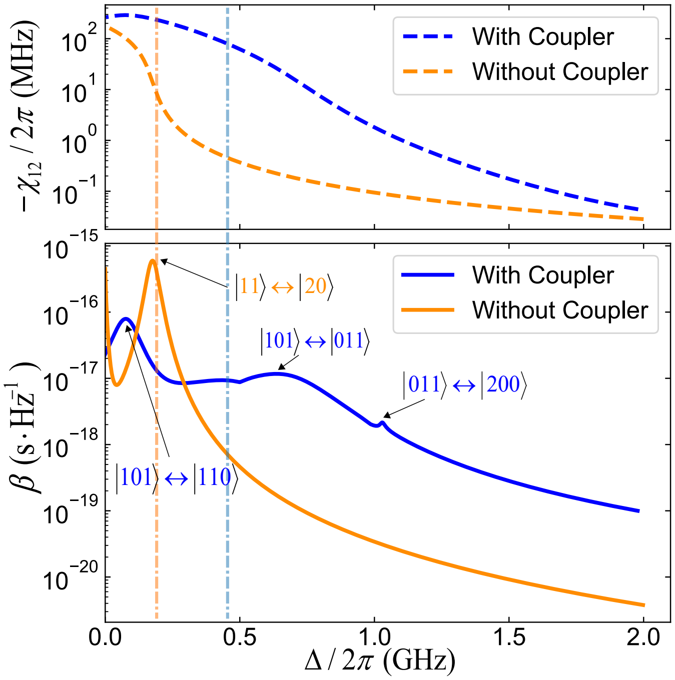


FIG. S3: Simulated ZZ-coupling (top panel) and $\beta_f$ (bottom panel) versus the frequency detuning $\Delta$. $\Delta = \omega_1 - \omega_2$ in the conventional scheme of using a tunable qubit (orange lines; parameters are from Ref. [4]); $\Delta = \omega_c - \omega_2$ in our scheme of using a tunable coupler (blue lines; parameter are from our device). The dashed vertical lines correspond to the maximum amplitude of the modulation pulses. In the case of using a tunable coupler, $\beta_f$ is nearly two-orders-of-magnitude smaller in the relevant region for two-qubit interactions, indicating enhanced adiabaticity.

Using the energy structure of our device, we calculate the effective ZZ coupling $\chi_{12}$ and the factor $\beta$ as a function of the coupler frequency, and compare them to the conventional scheme without a tunable coupler (Fig. S3). We find that, with the tunable coupler, the strongest $\beta$ experienced during the pulse is nearly two-orders-of-magnitude smaller than the conventional scheme, enabling faster and lower-leakage adiabatic controlled-phase gate. Also, we notice that there is a flat response region in $\beta$ after the coupler being tuned across the higher-frequency $Q_1$ during the process of our pulse. This suggests that our scheme has intrinsic robustness against instability of control parameters and pulse distortion.

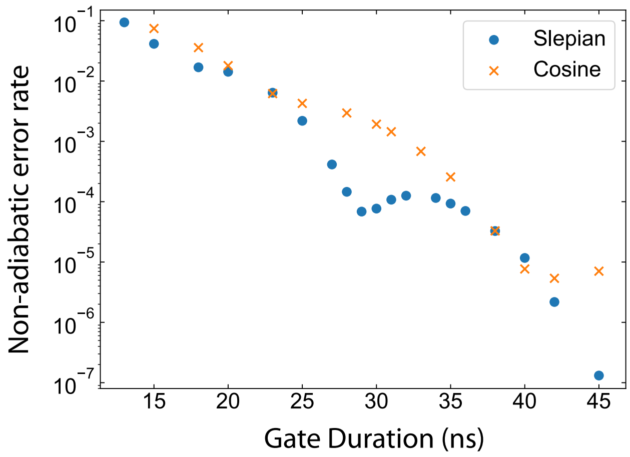


FIG. S4: Simulated non-adiabatic error rate with different gate duration using a cosine and more optimized pulse shape. The simulation is done with an additional 400 MHz Gaussian filter reshaping the pulse. There is no specific optimization for certain gate duration, and the reason for the dip shown around 30 ns in the Slepian case is unknown to us.

As shown in Fig. S4, we performed numerical simulations with the cosine pulse shape used in the experiment, which gives 0.18% non-adiabatic error rate with $\tau_{\text{gate}} = 30$ ns. We also tried alternative pulse shape similar to the original fast adiabatic CZ gate [2]. We find that non-adiabatic errors can be reduced to be below 0.01% with 30 ns gate time. This suggests the potential of this scheme when more coherent qubits become available and the signal distortion can be better remedied.

## III. ERROR ANALYSIS

### A. Single-qubit gate randomized benchmarking

We perform standard RB experiment for single-qubit gates on both qubits simultaneously. The results are shown in Fig. S5. The average single-qubit gate infidelity is 0.16% for $Q_1$ and 0.10% for $Q_2$.

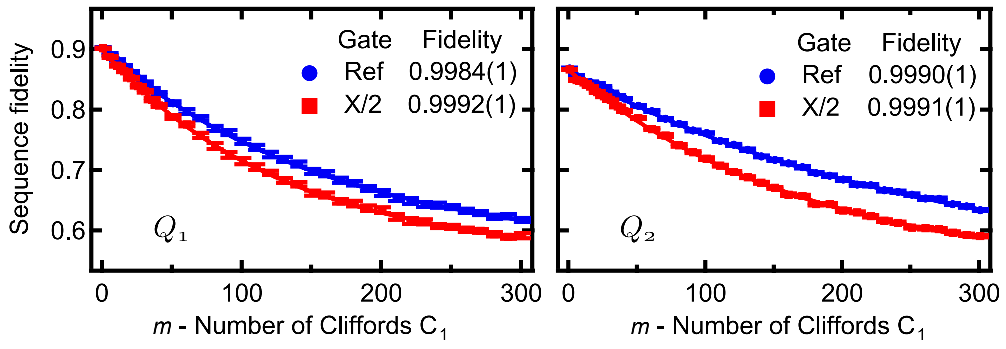


FIG. S5: Simultaneous single-qubit gate RB. Plotted are the sequence fidelity decay for the reference case and the interleaved $X/2$ case.

### B. Two-qubit gate randomized benchmarking

The calibrated two-qubit CZ gate is characterized by the conventional Clifford-based RB experiment, with the experimental sequences for both the reference and CZ-interleaved RB experiments shown in the inset of Fig. 3(a) in the main text. The reference RB experiment is performed by applying multiple random sequences composed of two-qubit Clifford gates $C_2$, followed by a recovery gate $C_r$ to invert the overall operation. The results are finally averaged over 100 random samples. The CZ-interleaved RB experiment is the same except for an additional CZ gate inserted to each Clifford cycle.

For the conventional two-qubit RB experiments on a two-level system, the ground state probability is measured as the sequence fidelity $P_{00} = \frac{3}{4}p^m_{\text{depolarized}} + \frac{1}{4}$, where $m$ is the number of Clifford gates and $p_{\text{depolarized}}$ is the depolarized error rate, giving the depolarized error per Clifford $r_{\text{depolarized}} = \frac{3}{4}\left(1 - p_{\text{depolarized}}\right)$. Thus, we perform exponential fit $F = Ap^m + B$ to the two decay curves in Fig. 3(a) in the main text to obtain the two decay constants, $p_{\text{ref}}$ and $p_{\text{int}}$, and then the error rate per Clifford, $r_{\text{ref}}$ and $r_{\text{int}}$, from $r = \frac{3}{4}(1-p)$. We can also extract the CZ gate error from $r_{CZ} = \frac{3}{4}(1 - p_{\text{int}}/p_{\text{ref}})$ and the CZ gate fidelity from $F_{CZ} = 1 - r_{CZ}$.

However, when the leakage errors are comparable to other depolarized errors, we need to consider a more complex model of the RB experiment. In this case, the total population occupation of the computational subspace $P_s$ changes as the number of Clifford gates $m$, $\Delta P_s/\Delta m = -r_{\text{leakage}}P_s + r_{\text{return}}(1-P_s)$, where $r_{\text{leakage}}$ is the leakage rate of the Clifford gate out of the subspace and $r_{\text{return}}$ is the total rate from the non-computational states returning back to the subspace. And thus, the final measured ground state probability can be expressed as $P_{00} = \left(\frac{3}{4}p^m_{\text{depolarized}} + \frac{1}{4}\right)P_s$, giving an offset of $\frac{1}{4}\frac{r_{\text{return}}}{r_{\text{return}}+r_{\text{leakage}}}$ for large number of Clifford gates $m$. Therefore, when the leakage rate $r_{\text{leakage}}$ are comparable to the leakage states returning back rate $r_{\text{return}}$, the two-qubit RB traces will not decay to 0.25 and have different offsets, as clearly observed in the experimental data in Fig. 3(a) in the main text.

### C. Frequency-dependence of coherence times

The energy relaxation time $T_1$ and pure dephasing time $T_\phi$ of qubit $Q_1$ and $Q_2$ are measured as a function of coupler frequency, with the experimental results shown in Fig. S6. These measured data are used for generating Fig. 3(b) in the main text. Their effective times during the CZ gate, $T_1^{\text{eff}}$ and $T_\phi^{\text{eff}}$, are obtained by integrating the error rates of energy relaxation (pure dephasing) over different coupler frequencies weighted by the actual half-period cosine pulse shape.

The effective/idling $T_1$ times are $6.54\mu/10.33\mu$s for $Q_1$, and $9.48\mu$s/$11.88\mu$s for $Q_2$. The effective/idling $T_\phi$ times are $0.49\mu$s/$8.86\mu$s for $Q_1$, and $7.21\mu$s/$17.63\mu$s for $Q_2$. Obviously, $T_1^{\text{eff}}$ and $T_\phi^{\text{eff}}$ are lower than their counterparts during idling periods ($T_1^{\text{idle}}$ and $T_\phi^{\text{idle}}$). In particular, the higher-frequency qubit $Q_1$ dephases drastically faster ($T^{\text{eff}}_{\phi,Q_1} \approx 0.5\ \mu$s), a consequence of the stronger interaction between the qubit and the less coherent coupler during the CZ pulse.

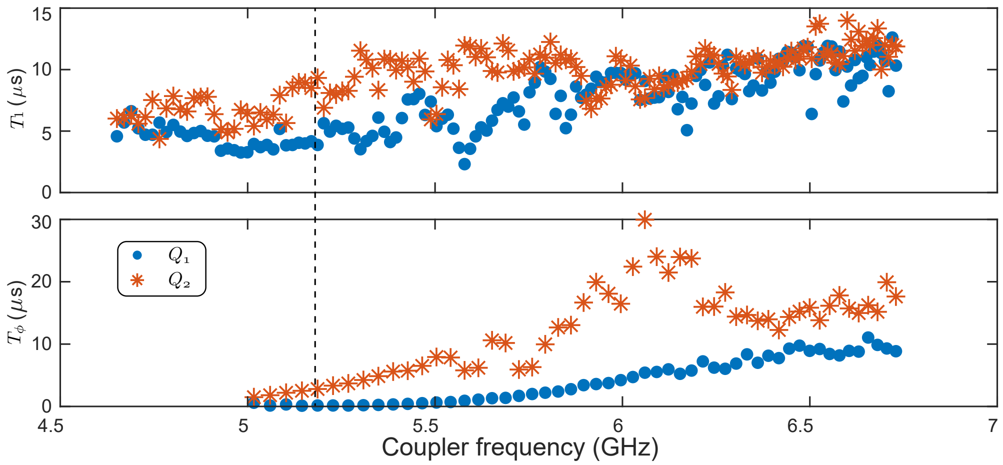


FIG. S6: Energy relaxation (top) and Gaussian pure dephasing (bottom) times v.s. the coupler frequency. The frequency corresponding to the maximum pulse amplitude is marked with the black dashed line.

### D. Pulse-induced error

Figure S7 shows the measured data used for generating Fig. 3(c) in the main text. The experiment is used to characterize the extra transitional errors induced by the CZ gate pulse. Note that the extracted transition rates per gate denote the additional errors caused by the CZ pulse, compared to the identity operation. These errors include two parts, additional energy relaxation during gate and transitions caused by the pulse-induced dynamic effect, in this case, the non-adiabatic effect. The experiment is performed on the four initial joint eigen-states $|00\rangle$, $|01\rangle$, $|10\rangle$, and $|11\rangle$, of the two qubits, with the experimental pulse sequence shown in Fig. S7(a) and the corresponding results shown in Fig. S7(b).

Note that the $|00\rangle$ state is supposed to give a flat response, because the adiabatic CZ gate should have almost no effect on the $|00\rangle$ state. However, we still observe a slight rising with pulse number in the measured population. One possible explanation is the CZ pulse may facilitate converting residual thermal or non-equilibrium excited-state populations to the ground state. The pulse-induced transitional error of $|00\rangle$ state is extracted from the difference of the slopes of the two linear fits. For the other three cases, the two population decay curves are fitted with an exponential decay function $F = Ap^m + B$, giving two decay constants $p_{\rm Id}$ and $p_{\rm CZ}$. The corresponding error rates are extracted by $r = 1 - p_{\rm CZ}/p_{\rm Id}$.

The extracted error per gate for each joint state is 0.005%, 0.185%, 0.196%, and 0.316%, respectively, as shown with orange bars in Fig. 3(c) in the main text. These pulse-induced transitional errors include additional energy relaxation during gate and other unwanted transitions coming from the non-adiabatic effects. The additional errors from shortening of energy relaxation times during CZ pulse are calculated by comparing the effective and idling $T_1$ times of the two qubits and shown with purple bars in Fig. 3(c) in the main text. The average difference between these transitional error rates and the $T_1$ contribution (orange versus purple bars in Fig. 3(c) in the main text), $(0.06 \pm 0.06)\%$, is thus the non-adiabatic errors. The number undershoots the simulation results presented in Fig. S4, possibly due to the fact that the repeated CZ pulses used in the experiment can produce interference effect, suppressing non-adiabatic errors.


[1] X. Li, T. Cai, H. Yan, Z. Wang, X. Pan, Y. Ma, W. Cai, J. Han, Z. Hua, X. Han, *et al.*, "Tunable coupler for realizing a controlled-phase gate with dynamically decoupled regime in a superconducting circuit," Phys. Rev. Applied **14**, 024070 (2020).

[2] J. M. Martinis and M. R. Geller, "Fast adiabatic qubit gates using only $\sigma_z$ control," Phys. Rev. A **90**, 022307 (2014).

[3] R. Barends, J. Kelly, A. Megrant, A. Veitia, D. Sank, E. Jeffrey, T. C. White, J. Mutus, A. G. Fowler, B. Campbell, *et al.*, "Superconducting quantum circuits at the surface code threshold for fault tolerance," Nature **508**, 500 (2014).

[4] M. Kjaergaard, M. E. Schwartz, A. Greene, G. O. Samach, A. Bengtsson, M. O'Keeffe, C. M. McNally, J. Braumüller, D. K. Kim, P. Krantz, *et al.*, "A quantum instruction set implemented on a superconducting quantum processor," arXiv: 2001.08838 (2020).

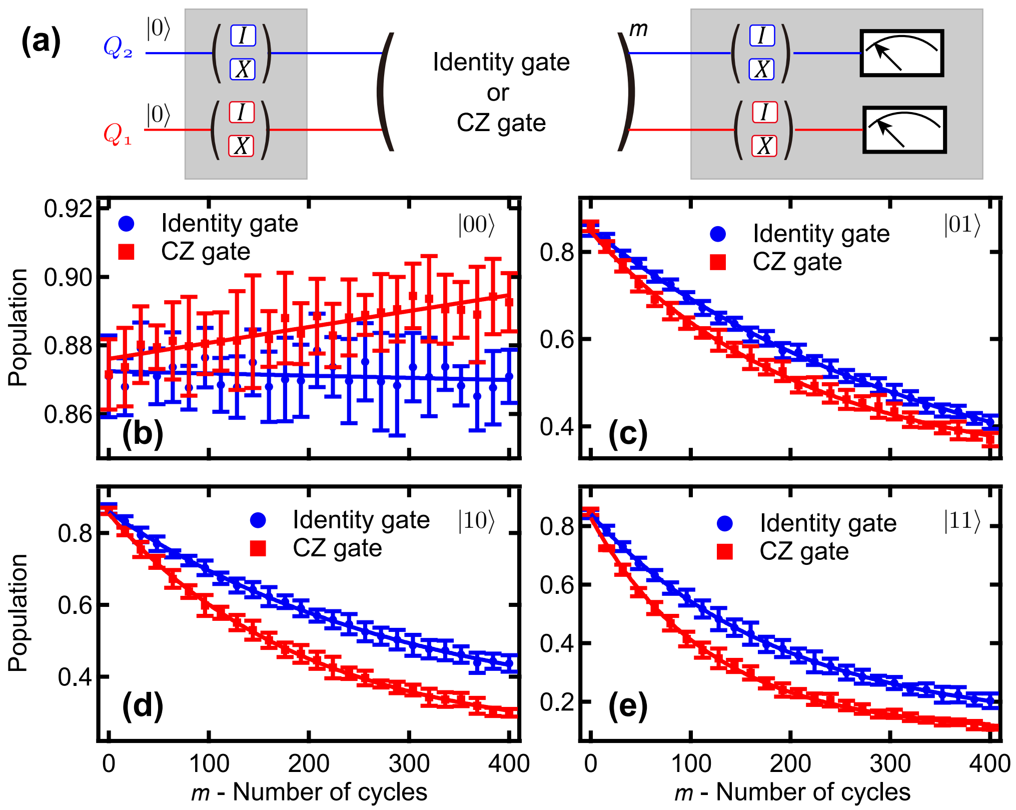


FIG. S7: The pulse-induced errors. (a) The pulse sequence for extracting the pulse-induced errors. A number of $m$ repeated CZ (or Identity) gates are applied. Optional $\pi$-pulses before the pulse train are used to prepare the state to $|00\rangle$, $|01\rangle$, $|10\rangle$, and $|11\rangle$. They are inverted back by symmetrically applied $\pi$-pulses after the pulse train before measuring the population of the system ground state. (b-e) The measured decay curves (markers) which are exponentially fitted (solid lines) except for the $|00\rangle$ case (linear fit).
